# Supplementary material for: Model-independent study of structure in $B^+\to D^+D^-K^+$ decays
Source: arXiv:2009.00025 source file (2020-12-17)
Supplement: Supplementary file 1 [file appendix.tex]

% ===============================================================================
% Purpose: appendix to the standard template: standard symbol alises from Ulrik
% Author: Tomasz Skwarnicki
% Created on: 2009-09-24
% ===============================================================================

%{\noindent\normalfont\bfseries\Large Appendices}
\section*{Appendices}

\appendix
